# Supplementary material for: Towards More Robust Interpretation via Local Gradient Alignment
Source: arXiv:2211.15900 source file (2022-12-07)
Supplement: Supplementary file 3 [file appendix_deprecated.tex]

% \begin{figure}[ht]
% \vskip 0.2in
% \begin{center}
% \centerline{\includegraphics[width=1.3\columnwidth]{figure/vis_attack-sup-lenet.png}}
% \caption{A visualization of attributions for original, randomly perturbed, and adversarially manipulated images .}
% \label{fig:visatt_cl-supp}
% \end{center}
% \vskip -0.2in
% \end{figure}


% \begin{figure}[ht]
% \vskip 0.2in
% \begin{center}
% \centerline{\includegraphics[width=1.3\columnwidth]{figure/vis_attack-sup-cifar101.png}}
% \caption{A visualization of the original and manipulated Gradient attribution for a CIFAR10 image with each model. The CE model corresponds to the $\ell_2$ and Hessian with $\lambda=0$. The AAM has been performed by PGD$_{\ell_\infty}(\epsilon=4)$}
% \label{fig:visatt_cr-supp1}
% \end{center}
% \vskip -0.2in
% \end{figure}

% \begin{figure}[ht]
% \vskip 0.2in
% \begin{center}
% \centerline{\includegraphics[width=1.3\columnwidth]{figure/vis_attack-sup-cifar102.png}}
% \caption{A visualization of the original and manipulated Gradient attribution for a CIFAR10 image with each model. The AAM has been performed by PGD$_{\ell_\infty}(\epsilon=4)$}
% \label{fig:visatt_cr-supp2}
% \end{center}
% \vskip -0.2in
% \end{figure}


% \begin{figure}[ht]
% \vskip 0.2in
% \begin{center}
% \centerline{\includegraphics[width=1.3\columnwidth]{figure/vis_attack-sup-resimg1.png}}
% \caption{A visualization of the original and manipulated Gradient attribution for an ImageNet image with each model. The AAM has been performed by PGD$_{\ell_\infty}(\epsilon=2)$}
% \label{fig:visatt_ir-supp1}
% \end{center}
% \vskip -0.2in
% \end{figure}

% \begin{figure}[ht]
% \vskip 0.2in
% \begin{center}
% \centerline{\includegraphics[width=1.3\columnwidth]{figure/vis_attack-sup-resimg2.png}}
% \caption{A visualization of the original and manipulated Gradient attribution for an ImageNet image with each model. The AAM has been performed by PGD$_{\ell_\infty}(\epsilon=2)$}
% \label{fig:visatt_ir-supp2}
% \end{center}
% \vskip -0.2in
% \end{figure}








%   \begin{sidewaystable}%
% \centering
% \caption{Quantitative results for every trained models.}
% \label{tab:appendix_rps1}
% \resizebox{\columnwidth}{!}{
% \input{table/table_appendix_rps1.tex}
% }
% \end{sidewaystable}


%   \begin{sidewaystable}%
% \centering
% \caption{Quantitative results for every trained models.}
% \label{tab:appendix_rps2}
% \resizebox{\columnwidth}{!}{
% \input{table/table_appendix_rps2.tex}
% }
% \end{sidewaystable}





%   \begin{sidewaystable}%
% \centering
% \caption{Quantitative results for every trained models.}
% \label{tab:appendix_saps1}
% \resizebox{\columnwidth}{!}{
% \input{table/table_appendix_saps.tex}
% }
% \end{sidewaystable}


% %   \begin{sidewaystable}%
% % \centering
% % \caption{Quantitative results for every trained models.}
% % \label{tab:appendix_saps2}
% % \resizebox{\columnwidth}{!}{
% % \input{table/table_appendix_saps2.tex}
% % }
% % \end{sidewaystable}





%   \begin{sidewaystable}%
% \centering
% \caption{Quantitative results for every trained models.}
% \label{tab:appendix_taps2}
% \resizebox{\columnwidth}{!}{
% \input{table/table_appendix_taps.tex}
% }
% \end{sidewaystable}




% %   \begin{sidewaystable}%
% % \centering
% % \caption{Quantitative results for every trained models.}
% % \label{tab:appendix_taps1}
% % \resizebox{\columnwidth}{!}{
% % \input{table/table_appendix_taps2.tex}
% % }
% % \end{sidewaystable}





%   \begin{sidewaystable}%
% \centering
% \caption{Quantitative results for every trained models.}
% \label{tab:appendix_ins_advacc}
% \resizebox{\columnwidth}{!}{
% \input{table/table_appendix_ins_advacc.tex}
% }
% \end{sidewaystable}
